# Supplementary material for: Tailoring hot-carrier distributions of plasmonic nanostructures through surface alloying
Source: arXiv:2311.09996 ancillary file (2023-11-16)
Supplement: Supplementary file 1 [file supporting-information.pdf]

# Supporting Information

## Tailoring hot-carrier distributions of plasmonic nanostructures through surface alloying

Jakub Fojt[1], Tuomas P. Rossi[2], Priyank V. Kumar[3], and Paul Erhart[1]

[1] *Department of Physics, Chalmers University of Technology, SE-412 96 Gothenburg, Sweden*
[2] *Department of Applied Physics, Aalto University, FI-00076 Aalto, Finland*
[3] *School of Chemical Engineering, The University of New South Wales, 2052 Sydney, NSW, Australia*

# Contents

**Supplementary Figures** **2**

S1. Normalized number of electrons and holes generated at the surface for different surface alloy compositions . . . 2
S2. Spatially resolved number of generated electrons and holes for various full-layer compositions 2
S3. Spatially resolved HC distributions for various full-layer compositions . . . 3
S4. Carrier distributions at the top surface of alloyed and unalloyed NPs . . . 4
S5. Number of HCs at the surface of the core-crown Ag–Pt NP for different surface alloy compositions and alloyants . . . 4
S6. Number of electrons and holes generated at the surface of alloyed and unalloyed NPs . . 5
S7. Geometry of surface alloys . . . 5

# Supplementary Figures

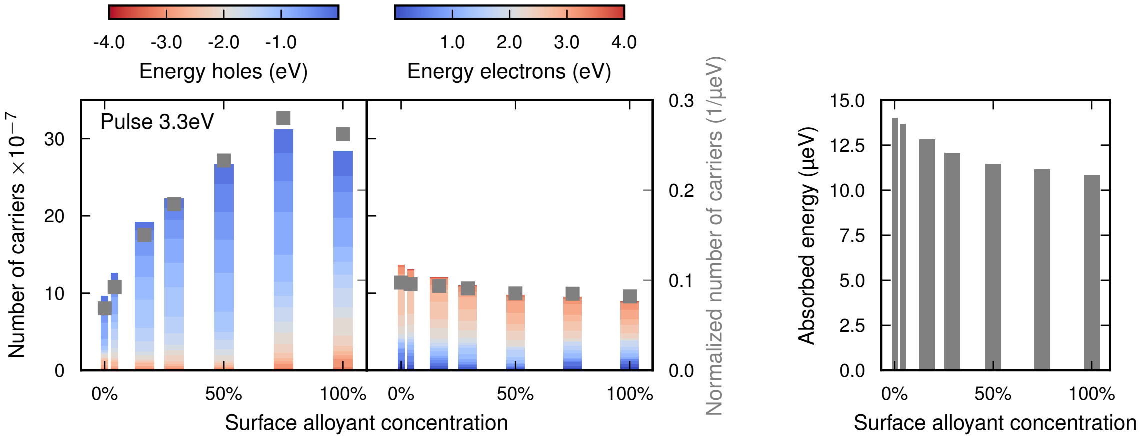


Figure S1: **Normalized number of electrons and holes generated at the surface for different surface alloy compositions.** The total number of HCs in the surface (left panel, bars), the total energy absorbed by the NP (right panel), and the former normalized by the latter (left panel, squares) are shown. The alloyant is Pt and the system was excited with a laser at the LSP peak (3.3 eV).

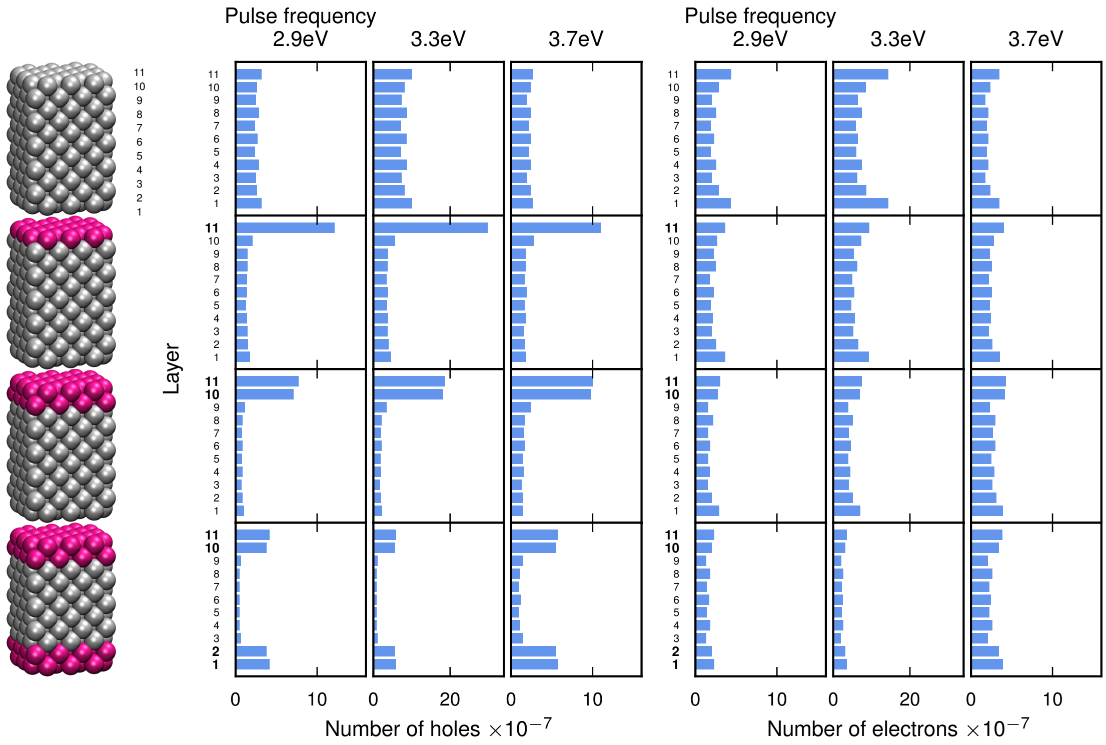


Figure S2: **Spatially resolved number of generated electrons and holes for various full-layer compositions.** Substitutions of Pt have been done in no layers, one top layer, two top layers, and two bottom and two top layers, as indicated by the highlights in the atomic structures. The non-alloyed NP has a relatively uniform spatial distribution of holes, and an electron distribution that is higher near the edges. Alloyed NPs have large numbers of holes localized to the alloy layers, while such a localization effect is lacking for electrons. Note the different scales for different pulse frequencies.

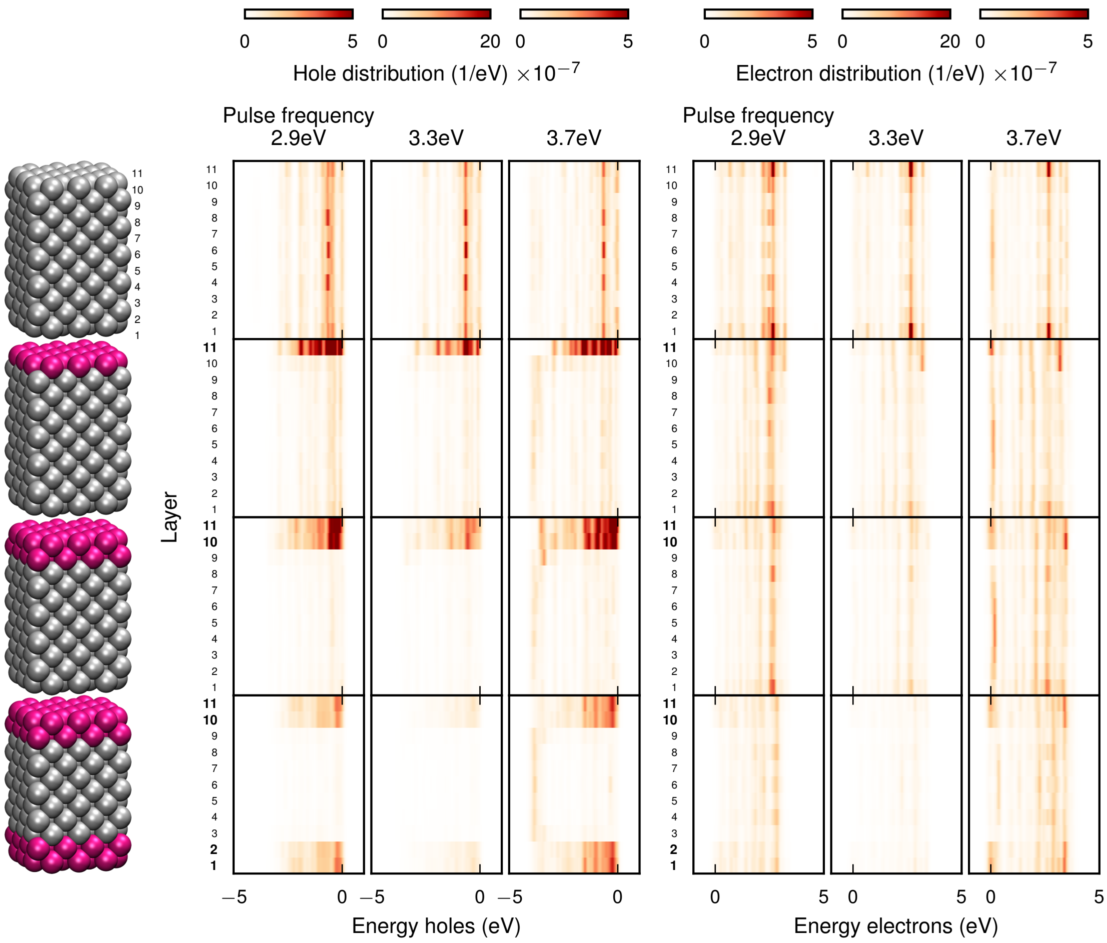


Figure S3: **Spatially resolved HC distributions for various full-layer compositions.** Substitutions of Pt have been done in no layers, one top layer, two top layers, and two bottom and two top layers, as indicated by the highlights in the atomic structures. For alloyed NPs, holes corresponding to the d-states of Pt are localized to the Pt layers, at energies between −2 and 0 eV. Such a localization effect is lacking for the electrons. For large pulse frequencies (3.7 eV), transitions from the d-band of Ag (−3.8 eV, holes) to the Fermi level (electrons) are possible, which is seen in the Ag layers. Note the different scales for different pulse frequencies.

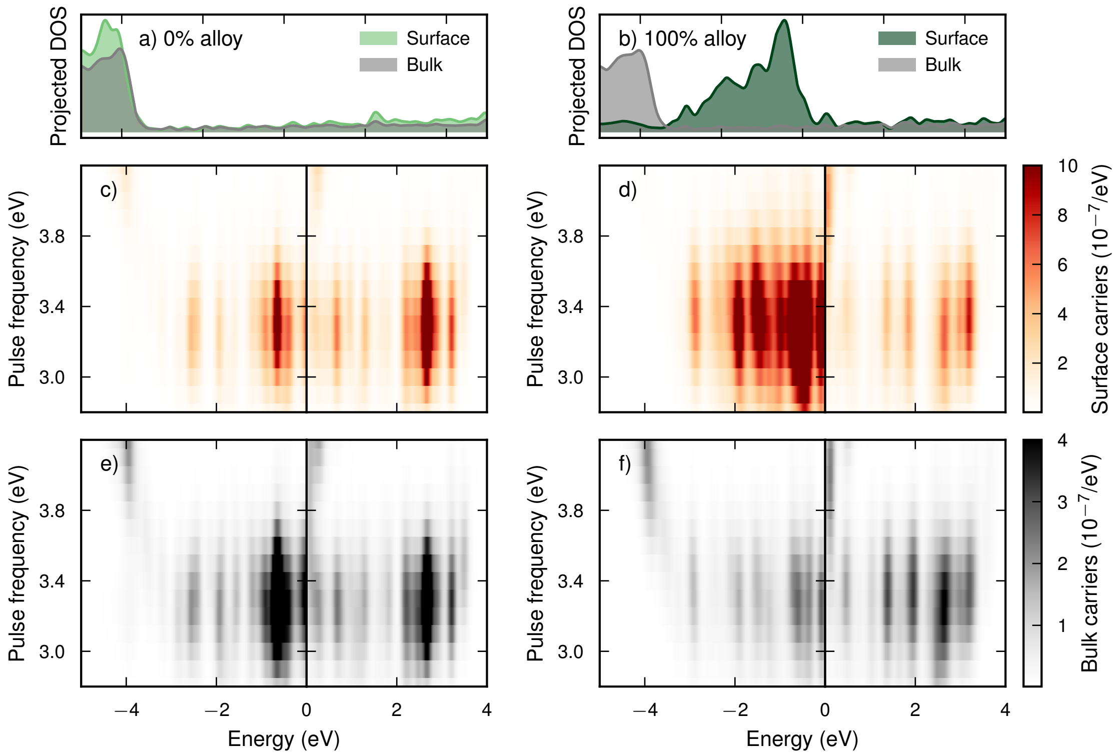


Figure S4: **Carrier distributions at the top surface of alloyed and unalloyed NPs.** (a-b) Projected densities of state, (c-d) surface and (e-f) bulk carrier distributions, for different exciting pulse frequencies. The alloyant is Pt. Note the different scales between surface and bulk.

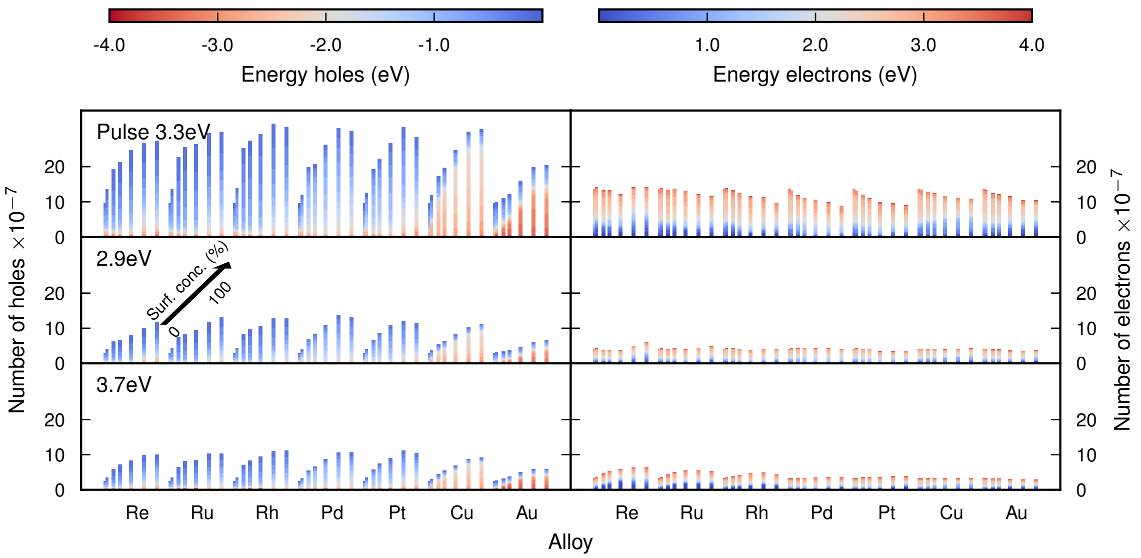


Figure S5: **Number of HCs at the surface of the core-crown Ag–Pt NP for different surface alloy compositions and alloyants.**

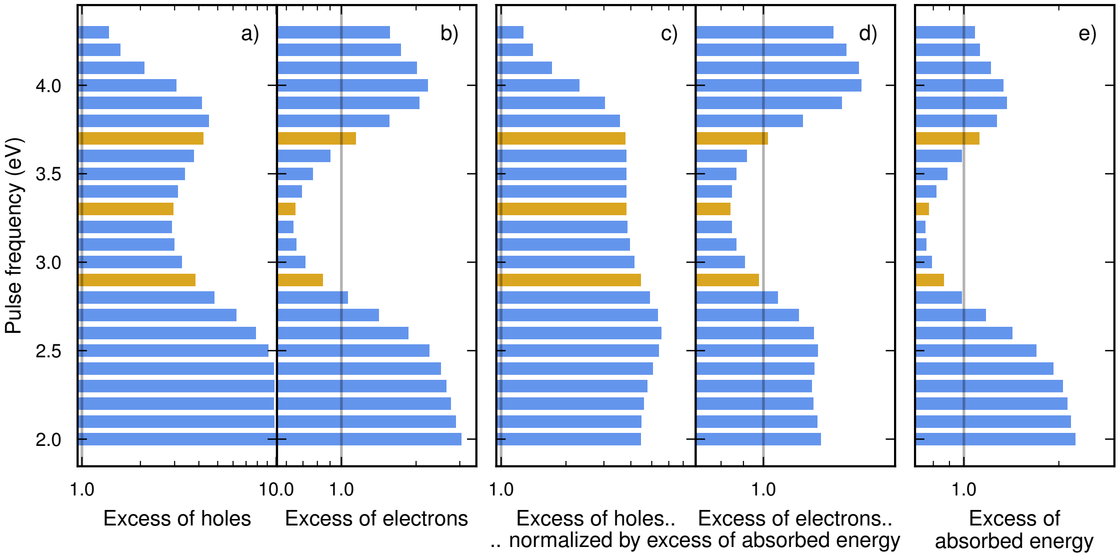


Figure S6: **Number of electrons and holes generated at the surface of alloyed and unalloyed NPs.** (a-b) The number of holes and electrons in the surface layer of the 100 % Pt surface alloy divided by the number of holes and electrons in the same surface of the non-alloyed NP. (b-c) The same quantities as in (a-b), scaled by the quantity in (e). (e) The amount of energy absorbed in the entire alloyed NP, divided by the amount of energy absorbed in the non-alloyed NP.

For pulse frequencies between 2.9 and 3.6 eV, the amount of energy absorbed in the alloyed NP is lower (e), due to lower oscillator strength. For the same frequencies, the number of electrons excited in the surface layer is decreased in the alloyed NP (b), even when compensating for the lower amount of energy absorbed (d).

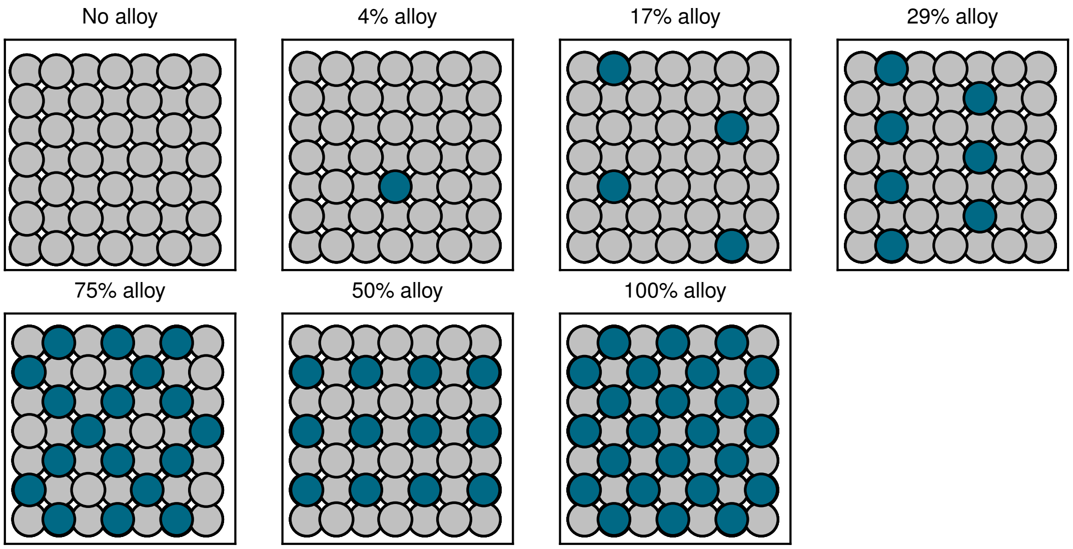


Figure S7: **Geometry of surface alloys.** View of the alloyed surface from the top.
